# Supplementary material for: Invidious Comparisons: Ranking and Selection as Compound Decisions
Source: arXiv:2012.12550 source file (2021-09-15)
Supplement: Supplementary file 1 [file Appendix.tex]

\section{notes on the literature of ranking and selection}
The literature on ranking and selection starts in 1950s, with \citeasnoun{Bahadur50} among the earliest authors to recognize that the ranking and selection is often more meaningful than test of homogeneity in many practical setting. One of the leading methodology, first appearing as the PhD thesis of \citeasnoun{Gupta56}, is called the subset selection inference (see also \citeasnoun{Gupta65}). 

Let $X_{ij}$ with $j = 1, \dots, m$ be an independent sample of size $m$ from population $\pi_1, \dots, \pi_n$ with distribution function $P_j$ indexed by a scalar parameter $\theta_j$. Let $\theta_{[1]} > \theta_{[2]} >\dots > \theta_{[n]}$ be the ordered parameters. The populations associated with $\theta_{[1]}, \dots, \theta_{[\tau]}$ is called the $\tau$-best populations, denoted as the set $R_0(P)$, our goal is to identify this group of populations. From a hypothesis testing point of view, this can be formulated as the $H_j: \theta_j < \theta_{[\tau]}$. Let the set $\hat R$ be the random selected set of individuals according to some decision rules. Let $PCS$ stands for the probability of the event of correct selection, which means that the $\tau-$best population is included in the selected set $\hat R$. For each fixed distribution $P = \{P_1, \dots, P_n\}$, we can evaluate 
\[
PCS(P) = P(R_0(P) \subseteq \hat R)
\]
and the confidence set of the $\tau-$best population is then defined as 
\[
\underset{P \in \mathcal{P}} {\inf} P(R_0(P)\subseteq \hat R) \geq 1- \alpha
\]
with $\mathcal{P}$ be a large family of distributions. \citeasnoun{Gupta56} develops a subset selection rule for the best population (i.e. $\tau = 1$) where $X_{ij}$ are random draws from a normal distribution with mean $\theta_i$ and common known variances. Most of the earlier development is based on exact calculation of Gaussian probability under very small $n$ for fixed $m$. For more complicated population distribution especially when the underlying population distribution is unknown, bootstrap methods have been proposed. More complications arise when the true parameters have ties, as pointed out by \citeasnoun{HM09} and \citeasnoun{Xie09}. 
Very recently, \citeasnoun{MRSW} propose a bootstrap based subset selection procedure that is robust to ties and has asymptotic coverage probability no less than $1-\alpha$ for a wide class of population distributions. One feature of the subset selection procedures is that the resulting selected set $\hat R$ is random, as well as the size of the selected set. If the values of $\theta$ are dense or when the sampling uncertainty is large, we may end up with a much larger selected list than the target $\tau$. However, if we fix the size of the selected set, then the resulting coverage probability may be too small to be useful in many applications.

\section{Conjugate prior for Normal model with unknown mean and variance}
Let $Y_{it} = \theta_i + \sigma_i \epsilon_{it}$ and $\epsilon_{it} \sim \mathcal{N}(0,1)$, omiting the individual index $i$, the likelihood can be written as 
\[
P(y_{1}, \dots, y_{T} | \theta, \sigma) = \frac{1}{(2\pi)^{T/2}}(\sigma^2)^{-T/2} \exp\Big(-\frac{1}{2\sigma^2} \Big[ (T-1)S + T(Y - \theta)^2\Big]\Big)
\]
where $Y$ and $S$ are respectively sample mean and variance of $\{y_1,\dots,y_T\}$. The random variable $(\theta,\sigma^2)$ follows normal-inverse-chi-squared distribution, which can be specified as 
\begin{align*}
g(\theta,\sigma^2) & = NI_{\chi^2}(\theta_0, \kappa_0, \nu_0,\sigma_0^2)\\
& = \mathcal{N}(\theta | \theta_0, \sigma^2/\kappa_0) \chi^{-2}(\sigma^2| \nu_0, \sigma_0^2)\\
& = \frac{\sqrt{\kappa_0}}{\sqrt{2\pi}} \frac{1}{\Gamma(\nu_0/2)}\Big(\frac{2}{\nu_0\sigma_0^2}\Big)^{-\nu_0/2} \sigma^{-1} (\sigma^2)^{-(\nu_0/2+1)} \exp\Big(-\frac{1}{2\sigma^2} [\nu_0 \sigma_0^2 + \kappa_0 (\theta_0 - \theta)^2]\Big)
\end{align*}
The marginal distribution of $\theta$ can be computed as 
\begin{align*}
g(\theta) & =  \int_0^{\infty} g(\theta,\sigma^2) d\sigma^2\\
& \propto \int (\sigma^2)^{-(\nu_0/2+\frac{1}{2}+1)}\exp(-A_0/2\sigma^2)d\sigma^2\\
& \propto A_0^{-(\nu_0+1)/2}\int x^{((\nu_0+1)/2 - 1)}\exp(-x)dx\\
& \propto A_0^{-(\nu_0+1)/2}\\
& = (\nu_0 \sigma_0^2 + \kappa_0(\theta - \theta_0)^2)^{-(\nu_0+1)/2}\\
& \propto \Big[ 1+ \frac{\kappa_0}{\nu_0 \sigma_0^2} (\theta - \theta_0)^2\Big] ^{-(\nu_0+1)/2}\\
& \propto t_{\nu_0}(\theta|\theta_0, \sigma_0^2/\kappa_0)
\end{align*}
where $A_0 = \nu_0 \sigma_0^2 + \kappa_0(\theta - \theta_0)^2$ and the third step follows from a change of variable $x = A_0/2\sigma^2$ and the last step shows that the marginal distribution of $\theta$ is a generalized $t$ distribution,
\[
\frac{\theta - \theta_0}{\sigma_0/\sqrt{\kappa_0}} \sim t_{\nu_0}
\]
This provides a mean to sample $(\theta,\sigma^2)$, that we can sample $\sigma^2$ from the inverse gamma distribution and then sample $\theta$ from the generalized $t$ distribution. The marginal distribution of $\theta$ also provides a mean to calculate $\theta_\alpha$. 

The posterior distribution of $(\theta,\sigma^2)$ is 
\begin{align*}
g(\theta,\sigma^2|y_1,\dots,y_T) & \propto  \Big[ \sigma^{-1} (\sigma^2)^{-(\nu_0/2+1)} \exp\Big(-\frac{1}{2\sigma^2} [\nu_0 \sigma_0^2 + \kappa_0 (\theta_0 - \theta)^2]\Big)\Big]\\
& \times \Big[( \sigma^2)^{-T/2} \exp\Big( -\frac{1}{\sigma^2} [(T-1)S + T(Y-\theta)^2]\Big) \Big]\\
& \propto \sigma^{-3} (\sigma^2)^{-(\nu_T/2)} \exp\Big( -\frac{1}{2\sigma^2} [\nu_T^2 \sigma_T^2 + \kappa_T(\theta_T - \theta)^2]\Big) \\
& = NI_{\chi^2}(\theta_T, \kappa_T,\nu_T, \sigma_T^2)
\end{align*}
with $\kappa_T = \kappa_0 + T$, $\nu_T= \nu_0 + T$, $\theta_T = (\kappa_0 \theta_0 + TY)/\kappa_T$ and $\sigma_T^2 = \frac{1}{\nu_T}(\nu_0 \sigma_0^2 + (T-1)S + \frac{T\kappa_0}{\kappa_T} (\theta_0 - Y)^2)$. Given the derivation of the marginal distribution for $\theta$, it is clear that the marginal posterior distribution for $\theta$ also follows a generalized $t$ distribution, more specifically 
\[
\frac{\theta - \theta_T}{\sigma_T/\sqrt{\kappa_T}} \sim t_{\nu_T}
\]
This provides a way to calculate $v_\alpha = \mathbb{P}(\theta \geq \theta_\alpha|Y,S)$ as the survival function of $t_{\nu_T}$ evaluated at $(\theta_\alpha - \theta_T)/\sigma_T/\sqrt{\kappa_T}$. It is also clear that the posterior mean of $\theta$ equals to $\theta_T$. 

The level curves reported in the examples in Section \ref{sec:UnknownVar} is constructed in the following way. We first draw a random sample of size n of $(\theta_i, \sigma_i^2)$ from the distribution $G$, which further allows us to generate a random sample $(y_{i1},\dots,y_{iT})$ for each individual. We then calculate sample mean and variances $(y_i,s_i)$ and based on these we calculate posterior tail probability $v_i =  \mathbb{P}(\theta \geq \theta_\alpha|y_i,s_i)$ and the posterior mean $pm_i = (\kappa_0 \theta_0 + Ty_i)/(\kappa_0 + T)$. Level curves are the contour plot of the sample of $v_i$ and $pm_i$.
